# Supplementary material for: Ultra-transient grating spectroscopy for visualization of surface acoustics
Source: arXiv:2510.10696 ancillary file (2026-11-05)
Supplement: Supplementary file 1 [file UTGS_v0710_supplementary.pdf]

# ***Supplementary Information for: Ultra-transient grating spectroscopy for visualization of surface acoustics***

**Tomáš Grabec<sup>1</sup>, Pavla Stoklasová<sup>1</sup>, Kristýna Repčák<sup>1</sup>, Jakub Kušnír<sup>1,2</sup>, David Mareš<sup>1</sup>, Martin Ševčík<sup>1</sup>, Petr Sedlák<sup>1</sup>, and Hanuš Seiner<sup>1,\*</sup>**

<sup>1</sup>Institute of Thermomechanics, Czech Academy of Science, Dolejskova 1402/5, 182 00 Prague, Czechia

<sup>2</sup>Faculty of Nuclear Science and Physical Engineering, Czech Technical University in Prague, Trojanova 13, 120 00 Prague, Czechia

\***Corresponding author:** hseiner@it.cas.cz (H. Seiner)

This Supplementary Information contains additional display items supporting the main text, and a Supplementary Discussion that brings details on the UTGS experiments described in the main text, and, using numerical simulations, it presents additional results supporting the explanation of the UTGS phenomenon and its features.

## Supplementary Data

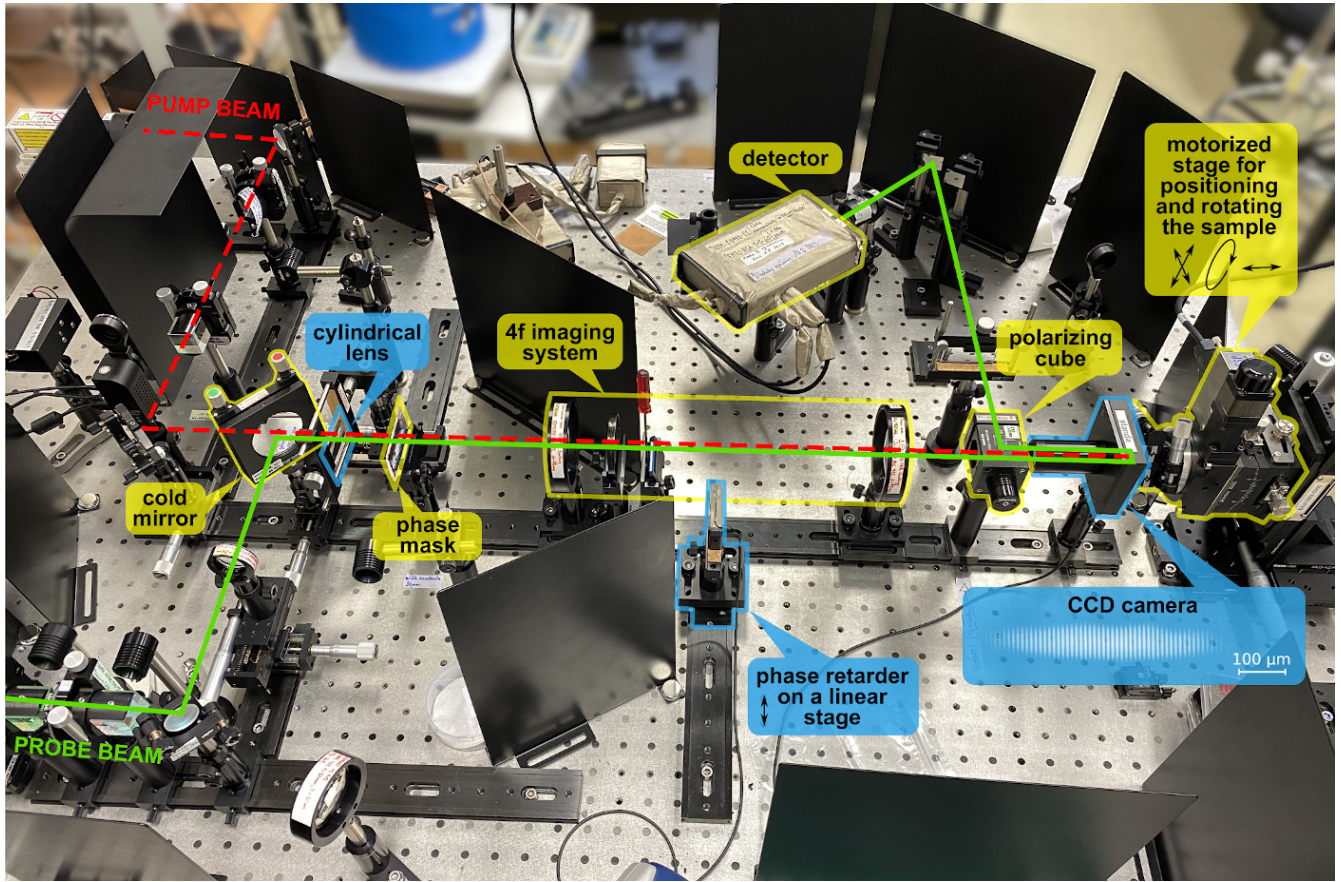

**Figure S1.** Photograph of the experimental setup used for UTGS experiments, complementing the schematics in Figure 1. For simplicity, both the pump and probe beams behind the phase mask are shown as single rays. The photograph shows also the CCD camera used to check and adjust the geometry of the interference pattern prior to the experiment, with a typical image of the probe beam pattern with high aspect ratio. For the measurement, the camera is replaced by a sample mounted onto a positioning stage, and the beam retarder is inserted into the optical path.

| sample denotation            | cut orientation [direction cosines] | the starting direction in TGS |
|------------------------------|-------------------------------------|-------------------------------|
| Ni (1 1 0)                   | (0.707; 0.707; 0)                   | [0; 0; 1]                     |
| Ni (3 1 1)                   | (0.905; 0.302; 0.302)               | [0; -1; 1]                    |
| Fe <sub>3</sub> Al (3 1 6)   | (0.482; 0.141; 0.865)               | [0.726; 0.489; -0.484]        |
| Fe <sub>3</sub> Al (1 2 7)   | (0.131; 0.310; 0.942)               | [-0.893; 0.450; -0.024]       |
| Fe <sub>3</sub> Al (10 5 11) | (0.639; 0.320; 0.700)               | [0.733; 0.024; -0.680]        |

**Table S1.** Exact orientations of the examined crystal cuts and the starting wave vector orientations (direction corresponding to zero propagation angle).

## Supplementary Discussion

### Time-domain signal processing

To extract the acoustic response of the sample from the measured signal and achieve the demonstrated similarity of the measured UTGS maps and calculated  $|G_{13}|$  maps, we use several main steps in the time-domain signal processing before the transition to the frequency-domain by employing the FFT:

1. We subtract the time-domain signal measured as background, measured by physically blocking the excitation laser at the beginning of its path and saving the signal recorded over the same amount of laser shots as the main measurement. This allows us to obtain the parasitic signals present in the main signal and subtract them. There are two main sources of the parasitic signals: ambient electromagnetic fields (such as GSM frequencies above 800 MHz) and burst signals generated by the electronics and pump laser. To minimize these influences, our detectors are physically wrapped in a shielding cloth, but there is still observable influence on the measured signal, which can be diminished by subtracting the background. Due to the extended measurement duration, some prominent background frequencies shift, and thus a better outcome was achieved by re-measuring of the background after each 5 measured angles (propagation directions) and associating each 'sample' signal to the closest background-signal measurement.
2. We omit the slow decay related to the thermal diffusion (shown in the time-domain signals in Figure 3 in the main text) by considering the numerical differences of the time-domain signal. This step reduces the influence of the low frequencies associated with the thermal decay.
3. We omit the initial 1.4 ns after the beginning of observed displacement – that is, after the beginning of the laser pulse. This removes the initial spike of the thermal-grating formation seen in the signal (even when considering only the numerical differences). The duration of 1.4 ns was chosen so that the resulting frequency-domain signals correspond to the acoustic-only response shown by the Green's function maps. However, it also closely corresponds to the duration for which the pump-laser pulse goes from 1% to 1% of the laser power, considering the time-domain Gaussian pulse profile with FWHM of 0.53 ns. Thus, the initial 1.4 ns corresponds to the time when the material response is influenced by the excitation – after that, it is the free response of the sample.

The effects of these steps are shown in Figure S2.

### Influence of extensive averaging and fine angle scanning

The importance of both the extensive averaging (recording 50,000 averages compared to 100) and very fine angular scanning (with the angular step of  $1^\circ$  instead of  $5^\circ$  or  $10^\circ$ ) is demonstrated in Figure S3.

There are two separate issues associated:

1. As documented by the Figure S3(a) showing a single signal, most of the fine, UTGS features are hidden in the noise without the extensive averaging. The difference between the first and second rows of measured maps—showing the effect of averaging—illustrates we could not detect the 'cliff' associated to the longitudinal limiting bulk wave without the extensive averaging. Even with the fine-tuned experimental setup, it is hidden in the noise and cannot be discerned. Some features connected to the shear-bands are present also in the low-averaged signal, although they are not recognizable in the single signal. The peak corresponding to the cuspidal point is not present at all in the low-averaged signal.

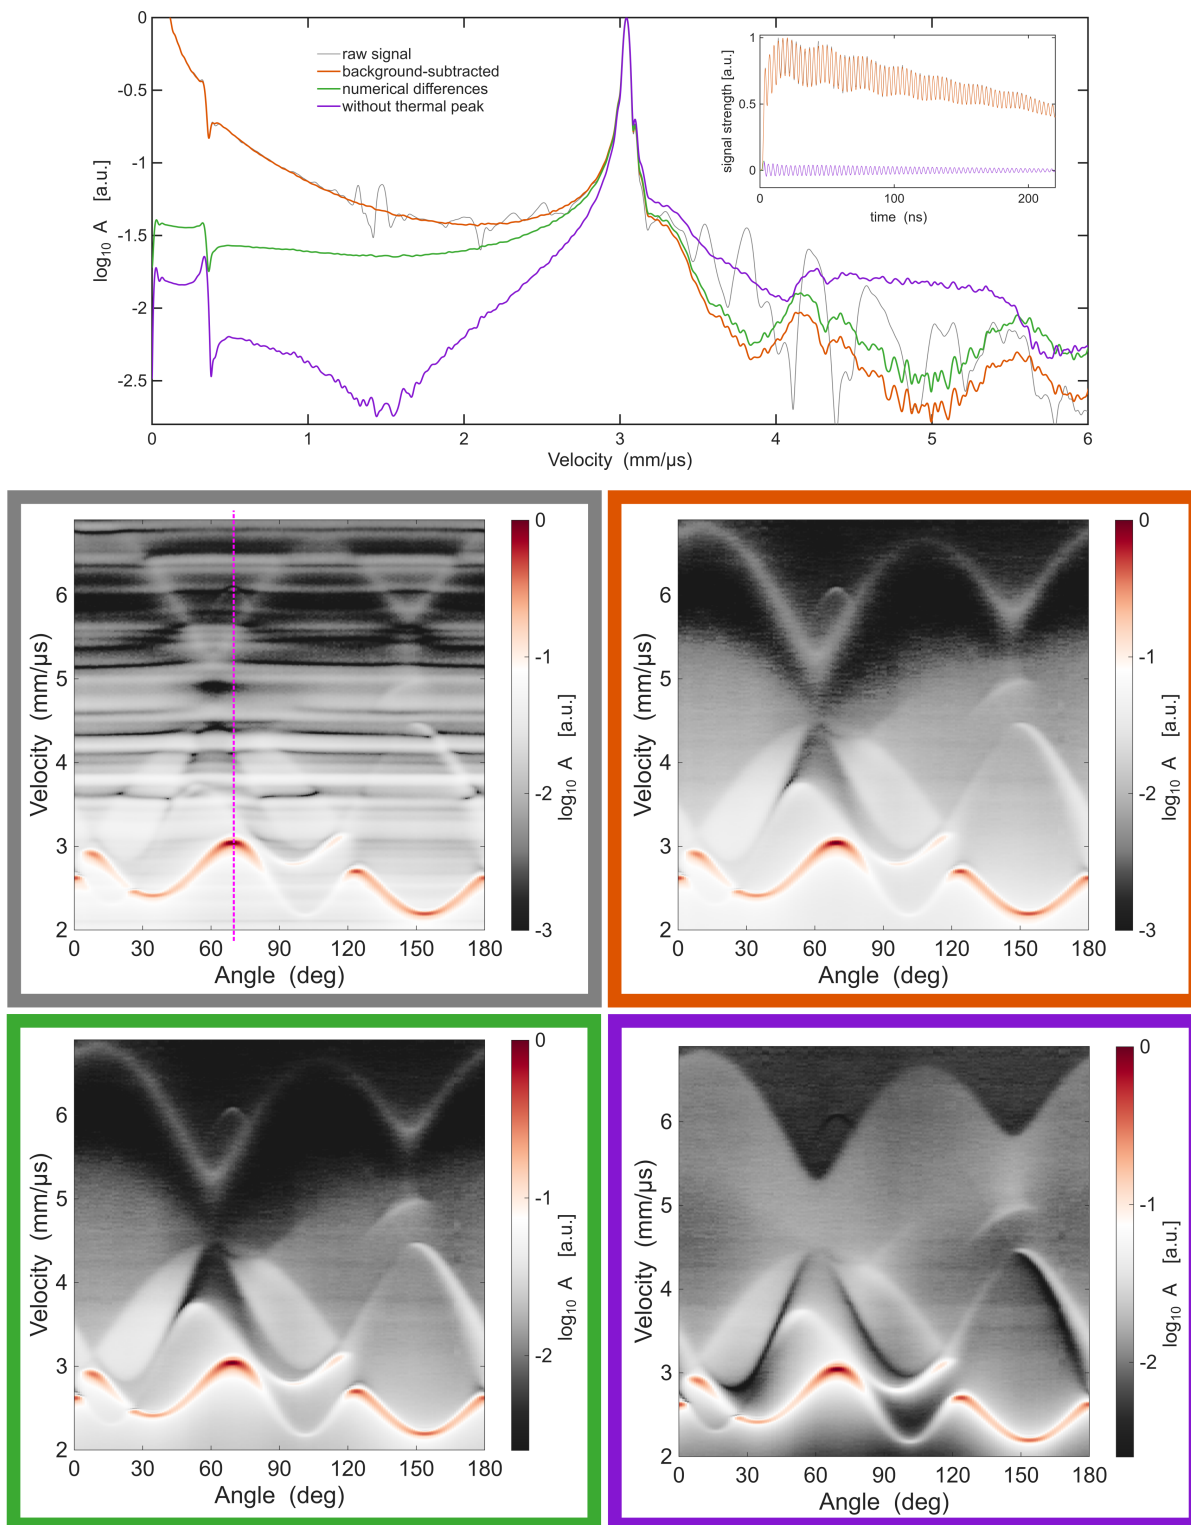

**Figure S2. Effects of time-domain signal processing steps.**

On top, frequency-domain signal at angle  $70^\circ$  of  $\text{Fe}_3\text{Al}$  (3 1 6) after various processing steps, with the corresponding time-domain signal shown in the inset): Starting with the raw (as-measured) signal (in gray), then after background subtraction (red), considering numerical differences (green), and finally after truncating first 1.4 ns (purple). The resulting maps of these processing steps are shown in the panels with corresponding color frame. The magenta line in the first map (gray frame) corresponds to the chosen angle of  $70^\circ$ .

2. On the other hand, the sequence of refinement in the angular scanning, corresponding to the columns of maps, shows that the shear-wave-related features are difficult to interpret with limited number of measured propagation directions. Although the signal of these shear-wave effects is stronger – and thus distinguishable from noise even in the low-averaged signal – it is not possible to interpret without the fine angular scanning. In the  $10^\circ$ -case, it is even complicated to judge the character of the SAW-related peak.

Of course, the rich information obtained by both extensive averaging and very fine angular scanning comes at the price of the measurement duration. The limitation on the potential speed of averaging comes from the pump-laser repetition rate, which is 1 kHz in our setup. The signal recording and averaging lowers the rate below 600 Hz – for simplicity, let's consider the lower boundary to be 500 averaged signals per second: For a single propagation direction, the measurement of 100 signals to be averaged takes 0.2 s, while that of the 50,000 averages takes 100 seconds. The net averaging time of 100 averages then starts at 3.6 s for map (b1), 7.2 s for map (b2), and 36 s for the map (b3). On the other hand, 50,000 averages take 30 minutes for map (c1), 1 hour for map (c2), and 5 hours for map (c3).

However, the real times are prolonged by the physical rotation of the sample, acquiring background signals (with an automated flipper blocking the pump laser), and saving data. Our setup runs in a conservative tempo, with the rotation of the sample and checking of various statuses adding another 20-30 seconds per angle. This could be, however, improved dramatically if necessary (and allowing for some amount of error present in the data), to a few seconds – which is not dramatic for the highly averaged signals, but crucial for fast angular scans with low averaging.

Ideal strategy for combining low- and high-averaged signals with sparse or fine angular scan then depends entirely on the goal of the particular measurement.

### **Influence of laser-pulse duration with respect to the measured frequency band**

To better understand various factors and processes in the TGS, both in excitation and detection of the sample response, we designed a coupled thermo-mechanical finite-element method (FEM) simulation of the process. Although this is yet unpublished work, it is based on a quasi-static simulation (omitting the dynamic processes connected to the acoustics) previously published by the authors, describing the heterodyne detection of a surface displacement excited by a harmonic thermal field.<sup>1</sup>

In Figure S4, we present the computational study of the laser-pulse duration and its influence on the simulated frequency spectrum in otherwise unchanged conditions. It is shown that the higher frequencies – containing the ultra-transient phenomena – are lowered in intensity compared to the main SAW peak. Even in our setup with the laser pulse with FWHM of 530 ps, the situation is not ideal and the ultra-transient phenomena would be stronger with a shorter pulse – ideally below 200 ps.

On the other hand, we can observe that the loss of intensity increases rapidly with increasing laser-pulse duration. Considering that the observed frequency is inversely tied to the chosen acoustic wavelength (of the interference pattern), the importance of this effect rises with lowering of the acoustic wavelength. Therefore, when measuring at wavelengths such as  $\lambda = 5 \mu\text{m}$ , the laser-pulse duration below 100 ps should be preferred.

There might arise a question of the energy absorption by the material, as the repetitive measurement requires to stay in the low-energy thermoelastic regime (not reaching material melting or even ablative regime). In this, however, the physics is in favor, as the energy required to reach the ablative regime is inversely proportional to the square root of laser-pulse duration.<sup>2</sup>

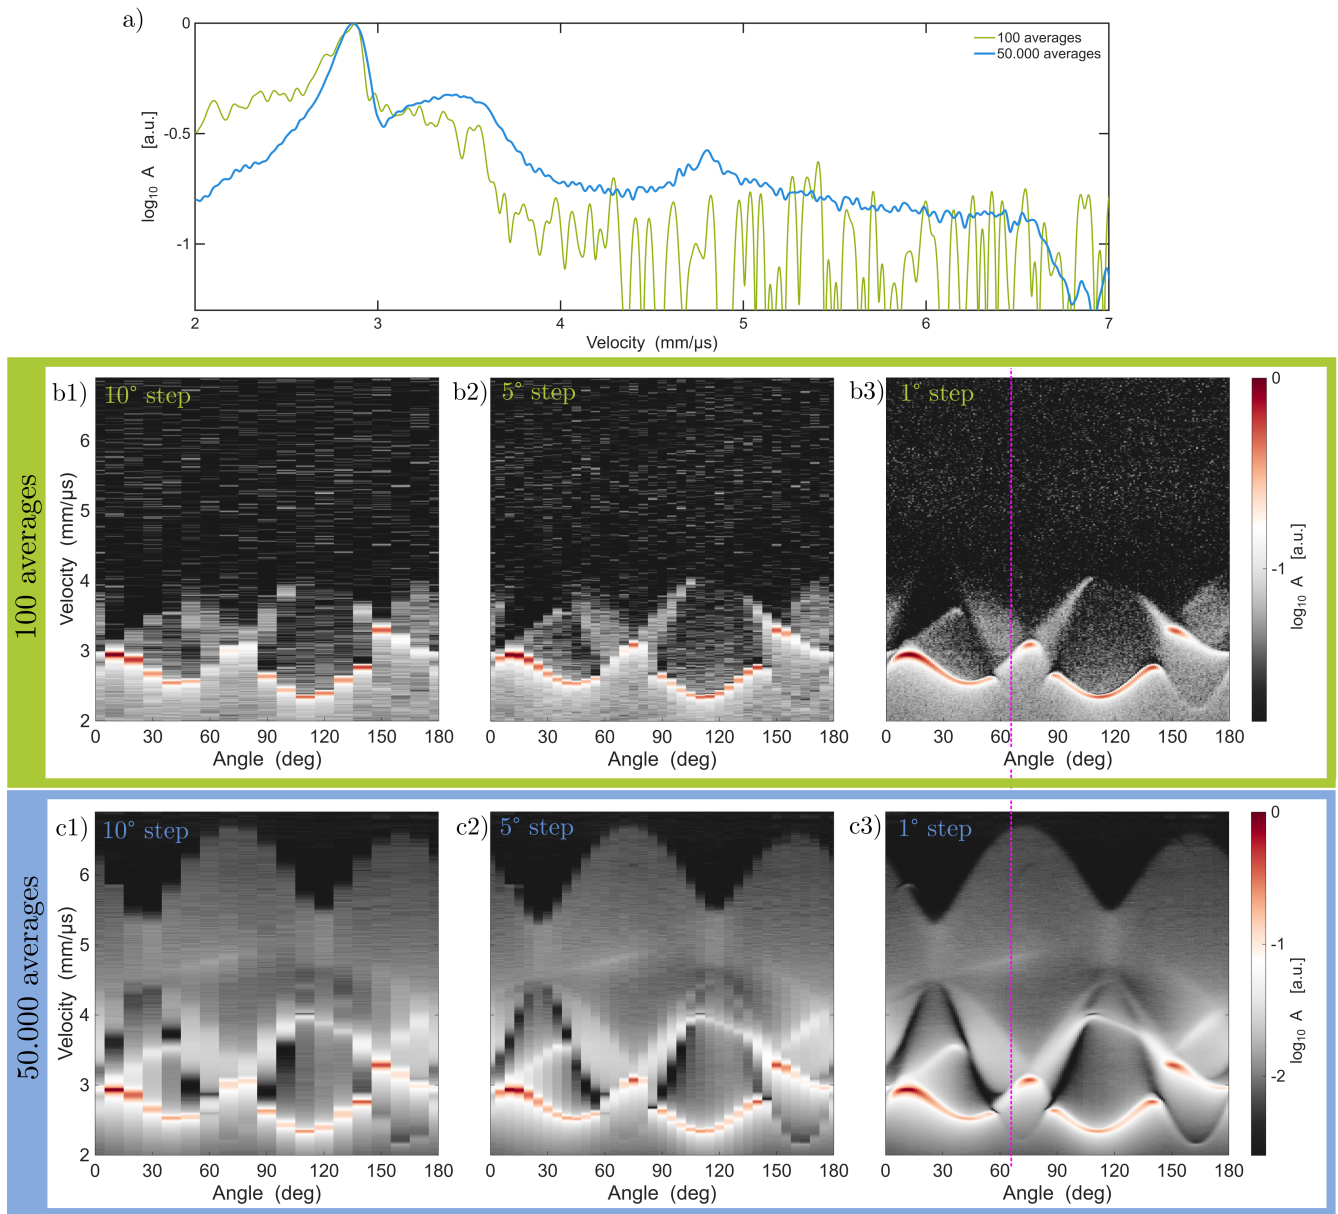

**Figure S3. Comparison of UTGS maps of  $\text{Fe}_3\text{Al}$  (1 2 7) with different level of averaging and angular step.** (a) Frequency-domain signal measured at angle  $66^\circ$  (denoted by magenta line in the third column of maps), comparing the resulting signal quality obtained by 100 and 50,000 averages (in green and blue, respectively), normalized to the main SAW peak. The row of figures (b1-b3) shows the maps obtained with 100 averages per angle, with varying angular step to 10, 5, and 1 degree of angle, respectively. The row below, (c1-c3), shows the maps obtained with 50,000 averages per angle with the same angular steps.

### Acoustic response as characterized by the FEM simulation

We can utilize the FEM simulation further to study only the acoustic response of the sample, omitting the thermal grating. This cannot be achieved simply by removing the thermal expansion, as that is necessary to launch the acoustic waves in the beginning. However, we can suppress the dynamic part of the response—the acoustic oscillations—and perform only a quasi-static simulation of the thermal grating.<sup>1</sup> Then, we can subtract the time-domain evolution of surface displacement due to the thermal grating from the full dynamic simulation to synthesize the surface displacement corresponding only to the

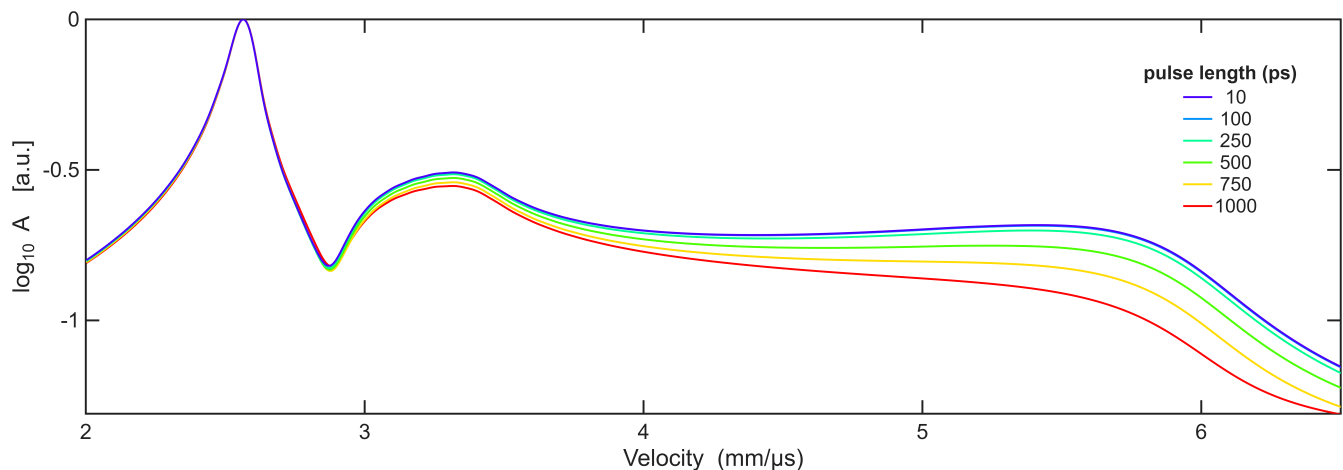

**Figure S4. Acoustic response of Ni (1 1 0) at 30° obtained by FEM with varying pulse lengths.**

Frequency-domain signal obtained from a FEM simulation of TGS, normalized to the main SAW peak, documenting the loss of intensity in higher frequencies (UTGS phenomena) with longer pulse length. While the differences between 10, 100, and 250 ps pulses (FWHM) are negligible, the relative intensity drops dramatically with longer pulses.

acoustic oscillations. The time-domain signal corresponding to these oscillations can be obtained using the method described in previously published work.<sup>1</sup> The result is shown in Figure S5, documenting excellent agreement with both the UTGS and  $|G_{13}|$  maps of the corresponding sample and its cut – Fe<sub>3</sub>Al (1 2 7).

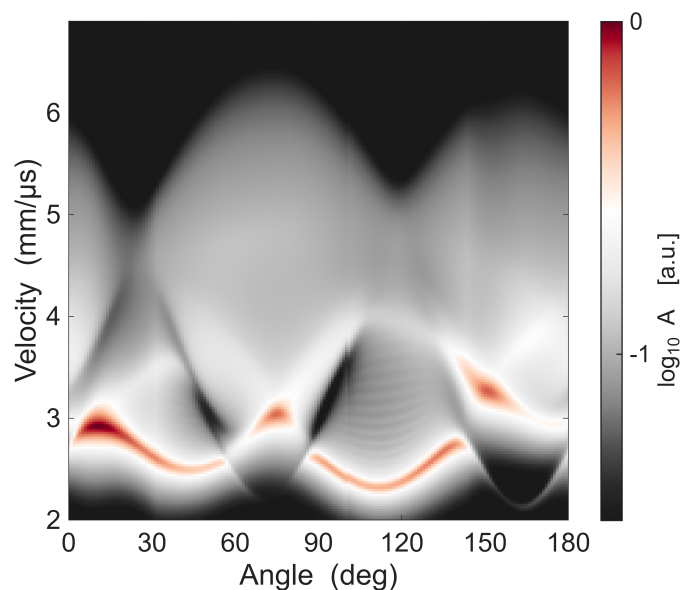

**Figure S5. Acoustic response of Fe<sub>3</sub>Al (1 2 7) sample obtained by FEM.** Frequency-angular dispersion map obtained by FEM simulation, synthesizing only the acoustic response – by removing the thermal grating (calculated separately) from the full, dynamic simulation of the TGS process. The result was a time-domain evolution of the displacement field solely representing the acoustic response. The simulated heterodyne detection was then performed on such displacement field.<sup>1</sup>

## References

1. Kušnír, J. *et al.* Apparent anisotropic thermal diffusivity measured in cubic single crystals by transient grating spectroscopy. *J. Appl. Phys.* **133**, DOI: [10.1063/5.0136850](https://doi.org/10.1063/5.0136850) (2023).
2. Ready, J. F. Effects Caused by Absorption of Laser Radiation at Opaque Surfaces. In Ready, J. F. (ed.) *Effects of High-Power Laser Radiation*, 67–125, DOI: [10.1016/B978-0-12-583950-1.50008-8](https://doi.org/10.1016/B978-0-12-583950-1.50008-8) (Academic Press, 1971).
